# Supplementary material for: Machine Learning the Energetics of Electrified Solid/Liquid Interfaces
Source: arXiv:2505.19745 ancillary file (2025-05-26)
Supplement: Supplementary file 1 [file SM.pdf]

# Supplemental Material: Machine Learning the Energetics of Electrified Solid/Liquid Interfaces

Nicolas Bergmann,† Nicéphore Bonnet,‡ Nicola Marzari,‡ Karsten Reuter,† and Nicolas G. Hörmann*,†

†*Fritz-Haber-Institut der Max-Planck-Gesellschaft, Faradayweg 4-6, D-14195 Berlin, Germany*

‡*Laboratory for Theory and Simulation of Materials, EPFL, Lausanne*

E-mail: hoermann@fhi.mpg.de

## Contents

**SI Computational Details** **S-3**

SI.1 Density-Functional Theory Calculations . . . . . . . . . . . . . . . . . . . . . . S-3

SI.1.1 Effective Screening Medium Calculations . . . . . . . . . . . . . . . . . . . . S-3

SI.1.2 Quantum ENVIRON Implicit Solvation Calculations . . . . . . . . . . . . . S-3

SI.2 Atomistic Simulations at Charged/Applied Field Conditions . . . . . . . . . . . S-4

SI.2.1 Molecular Dynamics . . . . . . . . . . . . . . . . . . . . . . . . . . . . . . S-5

**SII RAZOR Implementation** **S-5**

**SIII *Ab Initio* Thermodynamics** **S-6**

SIII.1 Obtaining Grand-Canonical Free Energies from Constant-Charge Molecular Dynamics . . . . . . . . . . . . . . . . . . . . . . . . . . . . . . . . . . . S-6
SIII.2 Obtaining Grand-Canonical Free Energies from Static Calculations . . . . . . . S-9
SIII.3 Adsorption Free Energies . . . . . . . . . . . . . . . . . . . . . . . . . . . . . .S-10

**SIV Modeling Charged Cu(100) Interfaces S-11**
SIV.1 Fermi-energy-derived Work Functions . . . . . . . . . . . . . . . . . . . . . . .S-11
SIV.2 $q$-derived Work Functions and Derivatives . . . . . . . . . . . . . . . . . . . .S-11
SIV.3 Machine Learning the Cu(100) System . . . . . . . . . . . . . . . . . . . . . . .S-16
SIV.3.1 Energies and Forces at the PZC . . . . . . . . . . . . . . . . . . . . . . . .S-16
SIV.3.2 Surface Dipole Moment and Born Effective Charges . . . . . . . . . . . . .S-17
SIV.4 Free Energy Contributions . . . . . . . . . . . . . . . . . . . . . . . . . . . . .S-18
SIV.4.1 Adsorbate Contributions . . . . . . . . . . . . . . . . . . . . . . . . . . . .S-18
SIV.4.2 OH Chemical Potential Contributions . . . . . . . . . . . . . . . . . . . . .S-20
SIV.5 Molecular Dynamics of adsorbed OH on Cu(100) . . . . . . . . . . . . . . . . .S-20
SIV.5.1 Double-Well Correction via Maxwell Construction . . . . . . . . . . . . . .S-20
SIV.5.2 Other Molecular Dynamics Results . . . . . . . . . . . . . . . . . . . . . .S-22

**SV Modeling $H_2O$ in an Electric Field S-24**
SV.1 Machine Learning $H_2O$ . . . . . . . . . . . . . . . . . . . . . . . . . . . . . .S-24
SV.1.1 Energies and Forces for the field free case . . . . . . . . . . . . . . . . . . .S-25
SV.1.2 Surface Dipole Moment and Born Effective Charges . . . . . . . . . . . . .S-25
SV.2 $H_2O$: Importance of $z$-projection in learning $P_z$ . . . . . . . . . . . . . . . . . . .S-28
SV.3 Geometry Optimization of $H_2O$ at an Applied Electric Field . . . . . . . . . . .S-28
SV.4 Molecular Dynamics of a $H_2O$ Molecule in an Electric Field . . . . . . . . . . .S-29
SV.5 $H_2O$ slab . . . . . . . . . . . . . . . . . . . . . . . . . . . . . . . . . . . . .S-30

**References S-31**

# SI Computational Details

## SI.1 Density-Functional Theory Calculations

We perform density-functional theory (DFT) calculations with the plane-wave Quantum ESPRESSO distribution[1,2], using the PBE exchange-correlation functional[3] and the GBRV 1.5 ultrasoft pseudopotentials[4]. We employ a plane-wave basis set with the cutoffs `ecutwfc`=45 Ry and `ecutrho`=360 Ry. The $k$-point grid for all molecular DFT calculations consists only of the Gamma-point. For periodic slab systems, we use Gamma-centered $(N_a \times N_b \times N_c)$ k-point grids, where the number of k-points $N_i$ in reciprocal direction $i$ is given by the real space cell length $l_i$ via the relation

$$N_i = \frac{3.621\,\text{Å}}{l_i} \times 12 \quad . \tag{S1}$$

For all surface calculations, we employ a symmetric slab setup, with each slab comprised of six symmetric layers, separated in $z$ direction by a vacuum region of at least 18 Å. The $k$-grid in the $c = z$ direction is set to $N_z = 1$, whilst the $a$ and $b$ directions are set using equation S1. For slab relaxations, we keep the two innermost slab layers frozen at the optimized bulk distance.

### SI.1.1 Effective Screening Medium Calculations

For the DFT calculations of $H_2O$ molecules in an electric field, we use the effective screening medium (ESM) method as implemented in Quantum ESPRESSO[5]. We set the ESM boundary conditions to the "metal-slab-metal" configuration (`esm_bc='bc2'`) and apply an $E_z$-field via the system parameter `esm_efield`. The effective screening region was consistently placed at a distance of 7 Å to the top-most atom in the $H_2O$ molecules.

### SI.1.2 Quantum ENVIRON Implicit Solvation Calculations

The slabs are embedded in the Quantum ENVIRON SCCS implicit solvent model[2,6] with a dielectric constant of $\varepsilon_r = 78.3$. The electron-density thresholds are set to $\rho_{\text{max}} = 0.005$ and $\rho_{\text{min}} = 0.0001$,

as in the "fitg03" model[6]. We choose the modified Poisson-Boltzmann model as a countercharge scheme, with an ion pair $z = \pm 1$, $c = 1\,\mathrm{mol/l}$, and $c_{\mathrm{max}} = 10\,\mathrm{mol/l}$.

## SI.2 Atomistic Simulations at Charged/Applied Field Conditions

With the second-order capacitive term assumed as configuration-independent, see main text, the atomistic simulations at charged or applied field conditions rely on the truncated Taylor expansion describing $E$ at the first-order term. The $0^{\mathrm{th}}$-order terms are then provided by the standard machine-learned interatomic potentials (MLIPs) trained on $E_0$ and $\mathbf{F}_0$ (see subsections SV.1.1 and SIV.3.1), while the first-order terms are provided by RAZOR-MLIP (see subsections SV.1.2 and SIV.3.2).

When considering atomic configurations $\alpha$ in the presence of an electric field oriented in the $z$ direction ($E_z$), the energy becomes

$$E^{\alpha}(E_z) = E_0^{\alpha,\mathrm{ML}} + \frac{\partial E^{\alpha}}{\partial E_z}\bigg|_{E_z=0}^{\mathrm{ML}} E_z = E_0^{\alpha,\mathrm{ML}} + P_z^{\alpha,\mathrm{ML}} E_z \tag{S2}$$

$$\mathbf{F}_i(E_z) = \mathbf{F}_{i,0}^{\mathrm{ML}} + \frac{\partial \mathbf{F}_i}{\partial E_z}\bigg|_{E_z=0}^{\mathrm{ML}} E_z = \mathbf{F}_{i,0}^{\mathrm{ML}} + \mathbf{Z}_i^{*,\,\mathrm{ML}} E_z\,, \tag{S3}$$

with $P_z^{\alpha}$ being the polarization in $z$ direction and $\mathbf{Z}_i^*$ the $z$-component, Cartesian vector of the Born effective charges.

When evaluating structures at an applied charge $q$, we solve

$$E(q) = E_0^{\alpha,\mathrm{ML}} + \frac{\partial E^{\alpha}}{\partial q}\bigg|_{q=0}^{\mathrm{ML}} q = E_0^{\alpha,\mathrm{ML}} + \left(\frac{P_z^{\alpha,\mathrm{ML}}}{\varepsilon_0 A} + \phi_0^{\mathrm{clean}}\right) q = E_0^{\alpha,\mathrm{ML}} + \phi_0^{\alpha,\mathrm{ML}} q \tag{S4}$$

$$\mathbf{F}_i(q) = \mathbf{F}_{i,0}^{\mathrm{ML}} + \frac{\partial \mathbf{F}_i}{\partial q}\bigg|_{q=0}^{\mathrm{ML}} q = \mathbf{F}_{i,0}^{\mathrm{ML}} + \frac{\mathbf{Z}_i^{*,\mathrm{ML}}}{\varepsilon_0 A} q\quad. \tag{S5}$$

Here, $\phi_0$ being the $\alpha$'s work function (divided by the electronic charge $q$).

In practice, the two MLIPs are combined by using the `LinearMixingCalculator` class in the Atomic Simulation Environment[7] (ASE), giving $E_0$ a weight of 1 and $\phi_0$ (or $P_z$) a weight of $q$ (or $E_z$). Note that we natively learn extensive quantities, which makes computations in a cell size different than the learning one straight-forward (the intensive bias in above equations is q/A).

### SI.2.1 Molecular Dynamics

We run $NVT$ molecular dynamics (MD) simulations at $T = 300\,\mathrm{K}$ with the Langevin thermostat as implemented in ASE[7]. We set the timestep to 1 fs. The Langevin thermostat requires setting a friction coefficient, which we set to 1.5 fs.

# SII RAZOR Implementation

Without loss of generality, we illustrate the RAZOR approach (Fig. 1 in the main text) for the NequIP neural network potential architecture[8]. In NequIP, the atomic features are mapped into irreducible representations of the O(3) symmetry group, with a key parameter being the "rotation order" $l = 0, 1, \ldots$. By representing $\varepsilon_i$ in eq. 1 of the main text with $l = 0$ in the `AtomwiseLinear` class, NequIP achieves the necessary rotational invariance prediction of $E$ and $\mathbf{F}_i$[8]. However, this implemented rotational invariance inherently prohibits predicting $P_z$ and $\mathbf{Z}_i^*$ using the same ansatz (see Figure S19) and it is necessary instead to learn a $z$-projected, equivariant vector quantity[9].
To achieve this, we represent $\mathbf{p}_i$ in the NequIP architecture with a rotation order $l = 1$, thus generating a Cartesian vector that possesses the required rotational equivariance. We incorporate the projection step by discarding the non-$z$ elements of $\mathbf{p}_i$ via

$$P_z^\alpha = \sum_{i\in\alpha} p_{z,i} = \sum_{i\in\alpha} \mathbf{e}_z^T \cdot \mathbf{p}(\mathbf{d}_i) \quad , \tag{S6}$$

which we implement in a new `AtomwiseProjection` class. Fig. S19 demonstrates that RAZOR indeed correctly learns and predicts the $z$-projected dipole $P_z^\alpha$ of an isolated water molecule.
A benefit from RAZOR is that it permits utilizing the same descriptors $\mathbf{d}_i$ used in the prediction of $E_0^\alpha$ and $\mathbf{F}_{0,i}$ to predict the first-order responses $P_z^\alpha$ and $\mathbf{Z}_i^*$, thus reducing the required additional computational overhead.
Next to the Cu(100) surface with adsorbed OH reported in the main text, we also demonstrate the validity and capabilities of RAZOR by applying it to an isolated water molecule and a water slab in

vacuum below. Specifically, these two test systems (see subsections SV.4 and SV.5) illustrate the analogy of the working principles of RAZOR for the description of systems in an uni-axial, electric field. For more information regarding computational parameters as well as the training structures, training procedures and the employed workflows, we refer to sections SIV and SV.4.

# SIII *Ab Initio* Thermodynamics

## SIII.1 Obtaining Grand-Canonical Free Energies from Constant-Charge Molecular Dynamics

As described in the main text, the total energy for a microstate $\alpha$ of a given interface composition $Z_i$ at charge $q$ in an implicit solvent environment is approximated as

$$E^{\alpha}(q) \approx E_0^{\alpha} + \phi_0^{\alpha} q + \frac{1}{2}\frac{q^2}{C_{\mathrm{el},0}} \quad , \tag{S7}$$

where $C_{\mathrm{el},0}$ refers to the electronic capacitance between the interface and the bulk electrolyte. We consider $C_{\mathrm{el},0}$ to be independent of $\alpha$, as it remains almost identical for different adsorbate configurations at identical interfacial chemical composition (e.g. $0.3\,\mu\mathrm{F\,cm^{-2}}$ for a $p(4\times4)$ OH-covered surface in a hollow site versus a bridge site).

From equ. (S7), we determine the charge-derivative

$$\frac{\partial E^{\alpha}(q)}{\partial q} = \phi^{\alpha}(q) = \phi_0^{\alpha} + \frac{q}{C_{\mathrm{el},0}^{\alpha}} \quad . \tag{S8}$$

The partition function $\mathscr{Z}$ for the interface configuration $Z_i$, defined via the Helmholtz free energy $F$

$$F^{Z_i} = -k_{\mathrm{B}}T \ln\left(\mathscr{Z}^{Z_i}\right) = -\frac{\ln\left(\mathscr{Z}^{Z_i}\right)}{\beta} \quad , \tag{S9}$$

$$\mathscr{Z}^{Z_i}(q) = \exp\left(-\beta F^{Z_i}(q)\right) = \sum_{\alpha} \exp\left(-\beta E^{\alpha}(q)\right) \quad , \tag{S10}$$

provides the occupation probability for a single state $\alpha$, via

$$p^{\alpha}(q) = \frac{\exp\left(-\beta E^{\alpha}(q)\right)}{\mathscr{Z}^{Z_i}(q)} \quad . \tag{S11}$$

Evaluating the derivative of $F^{Z_i}$ with respect to $q$

$$\begin{aligned} \frac{\partial F^{Z_i}(q)}{\partial q} &= -\frac{1}{\beta \mathscr{Z}^{Z_i}(q)} \frac{\partial \mathscr{Z}^{Z_i}(q)}{\partial q} = \sum_{\alpha} \frac{\exp\left(-\beta E^{\alpha}(q)\right)}{\mathscr{Z}^{Z_i}(q)} \frac{\partial E^{\alpha}(q)}{\partial q} \\ &= \sum_{\alpha} p^{\alpha}(q) \phi^{\alpha}(q) = \sum_{\alpha} p^{\alpha}(q) \left( \phi_0^{\alpha} + \frac{q}{C_{\mathrm{el},0}} \right) \end{aligned} \tag{S12}$$

corresponds to the work function average observed in the constant charge, canonical ensemble simulation $\sum_{\alpha} p^{\alpha}(q)\phi_0^{\alpha}$ plus the additional "potential drop" across the double layer that we do not explicitly simulate $\sum_{\alpha} p^{\alpha}(q) q C_{\mathrm{el},0}^{-1} = q C_{\mathrm{el},0}^{-1}$.

At any explicit charge value $Q$ we thus have

$$\left. \frac{\partial F^{Z_i}(q)}{\partial q} \right|_{Q} = \langle \phi^{\alpha} \rangle |_{Q} = \langle \phi_0^{\alpha} \rangle |_{Q} + \frac{Q}{C_{\mathrm{el},0}} \quad . \tag{S13}$$

As a result, evaluating the derivative of the free energy with charge becomes possible via the machine-learned predicted work function $\phi_0$ combined with canonical ensemble simulations at charge $Q$ via molecular dynamics.

Thus, we can insert eq. (S13) into a thermodynamic integration expression to get the $q$-dependent free energy expression $F^{Z_i}(q)$

$$\begin{aligned} F^{Z_i}(q) &= F_0^{Z_i} + \Delta F^{Z_i}(q) \\ &= \langle F^{\alpha} \rangle |_{0,T} + \int_0^q \left\langle \frac{\partial F^{\alpha}}{\partial q} \right\rangle \bigg|_{q',T} \mathrm{d}q' \\ &= \langle F^{\alpha} \rangle |_{0,T} + \int_0^q \langle \phi^{\alpha} \rangle |_{q',T} \, \mathrm{d}q' \quad . \end{aligned} \tag{S14}$$

In eq. (S14), $F_0^{Z_i}$ are the free energy contributions at q = 0. Different to the static case (section SIII.2, eq. (S22)), we use the time-averaged potential energies at the PZC $\langle E_0^{\alpha} \rangle$ at some constant

temperature $T$, which inherently include the capacitive enthalpic energy contributions[10]. This means that $F_0^{Z_i}$ is approximated via

$$F_0^{Z_i} = \langle F^{\alpha} \rangle|_{0,T} = \langle E_0^{\alpha} \rangle|_T + n_{\text{ads}}^{Z_i} \left( E_{\text{ZPE,ads}} - T S_{\text{vib,ads}} \right) \quad , \tag{S15}$$

using the zero point energy $E_{\text{ZPE}}$ and vibrational entropic contributions $S_{\text{vib}}$.

As of now, the energy $F^{Z_i}(q)$ represents the canonical free energy of the interfacial system at charge $q$. To obtain the grand-canonical energy $\Omega^{Z_i}(\phi_{\text{E}})$, the formation energy of the interface at a given potential, we need to Legendre transform $F^{Z_i}(q)$. For this we consider the formation energy $\tilde{F}^{Z_i}(q, \phi_{\text{E}})$, the cost to form the interface of charge $q$ while having taken out the charge $q$ from the the external circuit at an electrode potential $\phi_{\text{E}}$ as given by

$$\tilde{F}^{Z_i}(q, \phi_{\text{E}}) = F^{Z_i}(q) - q\phi_{\text{E}} \quad . \tag{S16}$$

In thermodynamic equilibrium, the interface configuration i.e. the observed charge $Q$ is the one that minimizes $\tilde{F}^{Z_i}(q, \phi_{\text{E}})$. At this $Q$, we see that $\phi$'s expectation value equals the electrode potential $\phi_{\text{E}}$

$$\begin{aligned} \left. \frac{\partial \tilde{F}^{Z_i}(q, \phi_{\text{E}})}{\partial q} \right|_Q &\stackrel{!}{=} 0 \\ \Leftrightarrow \left. \frac{\partial F^{Z_i}(q)}{\partial q} \right|_Q &= \phi_{\text{E}} \\ \langle \phi^{\alpha} \rangle|_Q &= \phi_{\text{E}} \quad , \end{aligned} \tag{S17}$$

which is consistent with the more common equilibrium condition that identifies the system-internal potential $\langle \phi^{\alpha} \rangle|_Q$ (e.g. via the work function) with the externally applied electrode potential. $\tilde{F}^{Z_i}$ for macroscopic electrodes evaluated at these equilibrium conditions is identical with the grand-canonical free energy

$$\Omega^{Z_i}(\phi_{\text{E}}) = F^{Z_i}(Q(\phi_{\text{E}})) - Q(\phi_{\text{E}})\phi_{\text{E}} \quad . \tag{S18}$$

Thus, by combining eqs. (S13), (S14), (S18), and (S17), we can derive a grand-canonical free energy expression from the constant charge simulation

$$\begin{aligned}
\Omega^{Z_i}(\phi_\mathrm{E}) &= F^{Z_i}(Q) - Q\phi_\mathrm{E} \\
&= F_0^{Z_i} + \Delta F^{Z_i}(Q) - Q\phi_\mathrm{E} \\
&= F_0^{Z_i} + \Delta\Omega^{Z_i}(\phi_\mathrm{E}) \\
&= \langle F^\alpha \rangle|_{0,T} + \int_0^Q \langle \phi^\alpha \rangle|_{q'} \,\mathrm{d}q' - Q\phi_\mathrm{E} \\
&= \langle F^\alpha \rangle|_{0,T} + \int_0^Q \langle \phi_0^\alpha \rangle|_{q'} \,\mathrm{d}q' + \frac{1}{2C_{\mathrm{el},0}}Q^2 - Q\phi_\mathrm{E} \\
&= \langle F^\alpha \rangle|_{0,T} + \int_0^Q \langle \phi_0^\alpha \rangle|_{q'} \,\mathrm{d}q' - Q\,\langle \phi_0^\alpha \rangle|_Q - \frac{1}{2C_{\mathrm{el},0}}Q^2 \quad .
\end{aligned} \tag{S19}$$

## SIII.2 Obtaining Grand-Canonical Free Energies from Static Calculations

Typically, *ab initio* thermodynamics are used to evaluate single, static chemical compositions $\alpha$. In this case, the canonical free energy $F^\alpha(q)$ can be approximated within a $2^{\mathrm{nd}}$ order Taylor Expansion via[11]

$$F^\alpha(q) = F_0^\alpha + \phi_0^\alpha q + \frac{1}{2}C_{\mathrm{el},0}^\alpha q^2 \tag{S20}$$

Within the CHE+DL approximation[11], $\Omega^\alpha(\phi_\mathrm{E})$ for a chemical system $\alpha$ is defined as

$$\Omega^\alpha(\phi_\mathrm{E}) = F_0^\alpha - \frac{C_{\mathrm{el},0}^\alpha}{2}(\phi_\mathrm{E} - \phi_0^\alpha)^2 \quad . \tag{S21}$$

Eqs. (S20) and (S21) both require an expression for $\alpha$'s free energy at zero charge conditions $F_0^\alpha$. We obtain $F_0^\alpha$ by augmenting the DFT potential energies $E_0^\alpha$ with vibrational enthalpic and entropic contributions[12]

$$F_0^\alpha = E_0^\alpha + n_\mathrm{ads}^\alpha \left(H_\mathrm{ads} - TS_\mathrm{vib,ads}\right) \quad , \tag{S22}$$

with $S_\mathrm{vib,ads}$ being the vibrational entropic contributions, and $H_\mathrm{ads}(T,p)$ being the sum of the zero-point energy $E_\mathrm{ZPE}^{*\mathrm{OH}}$ and heat capacitive free energy terms for a single adsorbate. As we are typically

interested in free energy differences between slabs of identical substrate composition, we ignore the vibrational contributions of the substrate metal atoms, as we assume that these cancel each other out.

## SIII.3 Adsorption Free Energies

For either the MD-averaged interface configurations $Z_i$ or the statically-evaulated compositions $\alpha$, we define the adsorption free energy $\Delta\Omega_{\text{ads}}^{\alpha\vee Z_i}(\phi_{\text{E}})$ by referencing $\Omega(\phi_{\text{E}})$ to the clean interface without adsorbates, normalized by the adsorbate coverage $\theta_{\text{ads}} = n_{\text{ads}}/n_{\text{sites}}$ [13]

$$\Delta\Omega_{\text{ads}}(\phi_{\text{E}}) = \frac{\Omega^{\alpha\vee Z_i}(\phi_{\text{E}}) - \Omega^{\text{clean}}(\phi_{\text{E}})}{\theta_{\text{ads}}^{\alpha}} - \mu_{\text{ads}}(T, \phi_{\text{E}}, c_{\text{ads}}) \quad . \tag{S23}$$

$\Delta\Omega_{\text{ads}}(\phi_{\text{E}})$ thus depends on the above-discussed free energy expressions of the adsorbed and clean interface, and the potential-, temperature-, and concentration-dependent chemical potential $\mu$ of the adsorbate species $\mu_{\text{ads}}$.

For our specific case of an OH adsorbate, we use standard CHE-referencing [14] for $\mu_{\text{OH}}$:

$$\begin{aligned}
\mu_{\text{OH}}(c_{\text{OH}}, \phi_{\text{E}}, T) &= \tilde{\mu}_{\text{H}_2\text{O}} - (\tilde{\mu}_{\text{H}^+} + \tilde{\mu}_{\text{e}^-}) \\
&= G_{\text{H}_2\text{O}}^{\text{ref}} - \left(\frac{1}{2}G_{\text{H}_2}^{\text{ref}} + k_{\text{B}}T\ln(c_{\text{H}+}) - e\left(\phi_{\text{E}} - \phi_{\text{H}^+}^{\text{ref}}\right)\right) \\
&= G_{\text{H}_2\text{O}}^{\text{ref}} - \frac{1}{2}G_{\text{H}_2}^{\text{ref}} + k_{\text{B}}T\ln(10) \times \text{pH} + e\left(\phi_{\text{E}} - \phi_{\text{SHE}}^{\text{ref}}\right) \\
&= \mu_{\text{OH}}^{\circ} + k_{\text{B}}T\ln(10) \times \text{pH} + e\left(\phi_{\text{E}} - \phi_{\text{SHE}}^{\text{ref}}\right) \quad ,
\end{aligned} \tag{S24}$$

with $\phi_{\text{SHE}}^{\text{ref}} = 4.44\,\text{V}$. In eq. (S24), we have split $\mu_{\text{OH}}$ into two parts: A reference chemical potential $\mu_{\text{OH}}^{\circ}$ and the dependencies on $c_{\text{ads}}$, $T$, and $\phi_{\text{E}}$. We define adsorption energies that only take $\mu_{\text{OH}}^{\circ}$ into account as

$$\Delta\Omega_{\text{ads}}^{\circ}(\phi_{\text{E}}) = \frac{\Omega^{\alpha\vee Z_i}(\phi_{\text{E}}) - \Omega^{\text{clean}}(\phi_{\text{E}})}{\theta_{\text{ads}}^{\alpha}} - \mu_{\text{ads}}^{\circ} \quad . \tag{S25}$$

While shown here for the grand-canonical case of $\Omega(\phi_{\text{E}})$, the same relations hold true for the

canonical case of $F(q)$:

$$\Delta F_{\text{ads}}(q) = \frac{F^{\alpha \vee Z_i}(q) - F^{\text{clean}}(q)}{\theta^{\alpha}_{\text{ads}}} - \mu_{\text{ads}} \tag{S26}$$

$$\Delta F^{\circ}_{\text{ads}}(q) = \frac{F^{\alpha \vee Z_i}(q) - F^{\text{clean}}(q)}{\theta^{\alpha}_{\text{ads}}} - \mu^{\circ}_{\text{ads}} \quad . \tag{S27}$$

We show the DFT results for the individual contributions to $\mu_{\text{OH}}$ and $F_0$ in subsection SIV.4.

# SIV Modeling Charged Cu(100) Interfaces

## SIV.1 Fermi-energy-derived Work Functions

In conventional DFT slab setups, the work function at the point of zero charge $\phi_0$ can be determined by taking the difference between the potential in the bulk electrolyte $\phi_{\text{bulk}}$ and the Fermi energy of the atomic system $E_{\text{F}}$. Within Quantum Espresso and Quantum ENVIRON[2,6], these values are given by the outputs `fermi_energy` and `fermi_energy_env_shift`, respectively.

$$\phi_0 = \frac{e\phi_{\text{bulk}} - E_{\text{F}}}{e} = -(\texttt{fermi\_energy} + \texttt{fermi\_energy\_env\_shift}) \tag{S28}$$

From Fig. S1, we see that $\phi_0$ for the Cu(100) symmetric slab setup converges at $n_{\text{layers}} \geq 6$.

## SIV.2 *q*-derived Work Functions and Derivatives

Evaluating DFT energies in symmetric slab setups under charged conditions is straight forward in implicit model environments[11,15,16], where one obtains in general:

$$\phi_0 = \left.\frac{\partial E}{\partial q}\right|_{q=0} \tag{S29}$$

Here, we chose to do calculations at $q = \pm 0.25\,\text{e}$, which for a symmetric $(4 \times 4)$ cell of Cu(100) results in a charge per surface atom of $\approx 0.008e$ and surface charge density of

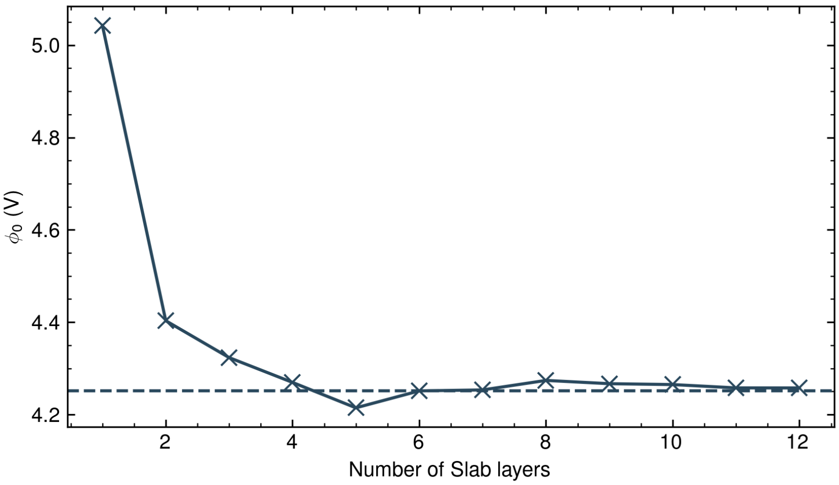


Figure S1: DFT-calculated work function $\phi_0$ for a clean Cu(100) slab whilst varying the number of Cu layers.

$$\frac{0.25\,\mathrm{e}\times 1.6022\times 10^{-19}\,\mathrm{C/e}}{2\times 105\,\mathring{\mathrm{A}}^2} = 1.907\times 10^{-22}\,\mathrm{C}/\mathring{\mathrm{A}}^2 = 1.907\,\mu\mathrm{C/cm}^2. \tag{S30}$$

Then, the work function is determined by evaluating the derivative of a quadratic polynomial fit through $E\left(q \in \{-0.25, 0.0, 0.25\}\right)$ at $q = 0$.

In Fig. S2, we see that this approach results in an almost exact recreation of the Fermi-energy-derived work function, with a maximum error of 2 meV.

To then transform $\phi_0$ into the surface dipole moment $P_z$, we use the Helmholtz equation[17,18]

$$P_z^\alpha = \varepsilon_0 A \left(\phi_0^\alpha - \phi_0^{\mathrm{ref}}\right) = \varepsilon_0 A \left( \left.\frac{dE^\alpha}{dq}\right|_{q=0} - \phi_0^{\mathrm{ref}} \right) . \tag{S31}$$

By the same logic, we get the born effective charges $\mathbf{Z}_i^*$ for each atom $i$ in the structure $\alpha$, by considering the condition from[16]

$$\left.\frac{\partial \mathbf{F}_i}{\partial q}\right|_{q=0} = -\frac{\partial \phi_0^{\mathrm{Fermi}}}{\partial \mathbf{r}_i} . \tag{S32}$$

We show that this assumption is true in Figs. S3 and S4, by explicitly displacing individual atoms $i$ along the three Cartesian dimensions and comparing the finite-difference-determined values

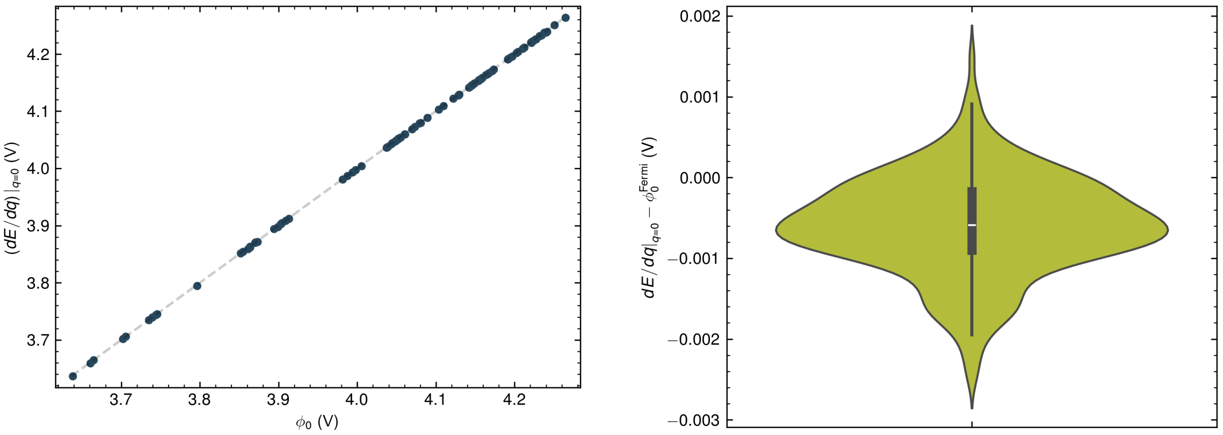


(a) $\phi_0$ determined via the Fermi energy on the $x$ axis versus $\partial E/\partial q$ on the $y$ axis.

(b) Violinplot of the difference between fermi- and energy-derived work functions. The majority of errors are below 1 mV.

Figure S2: Checks that energy-derived and Fermi-energy-derived work functions are consistent.

$d\phi_0/d\mathbf{r}_i$ to $-d\mathbf{F}_i/dq$ at $d\mathbf{r}_i = 0$.

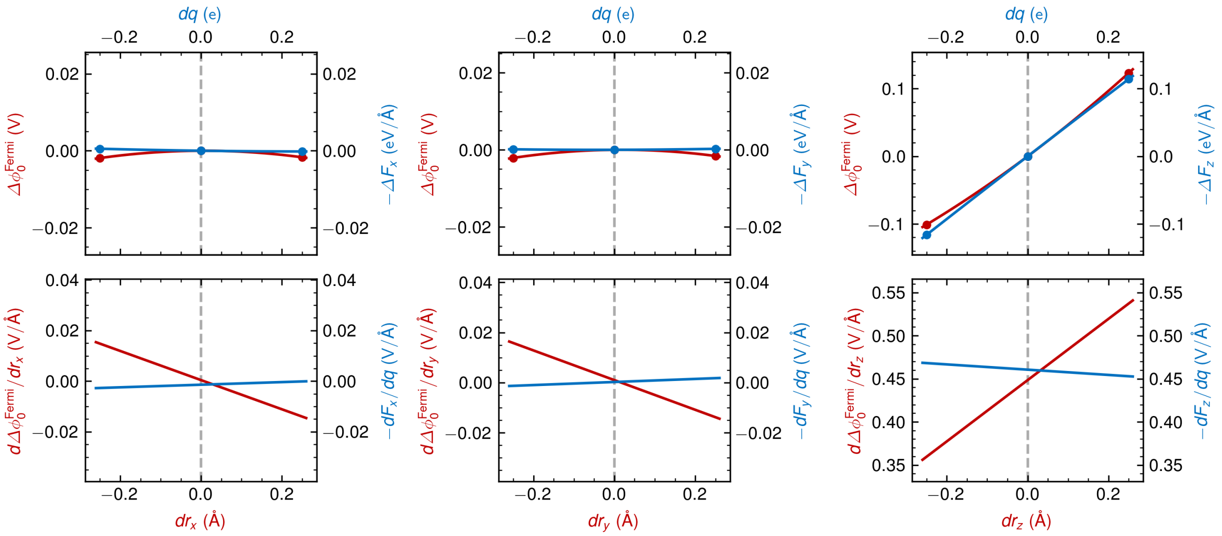


Figure S3: For the three Cartesian dimensions (from left to right: $x$, $y$, and $z$): $\Delta F(q)$ vs $\Delta\phi_0^{\mathrm{Fermi}}(r)$ for an adsorbed hydroxide molecule on the fourfold hollow site on a Cu(100) surface. $\Delta$ refers to the difference of the respective properties at $dq = dr = 0$. In the top row, we show $\phi^{\mathrm{Fermi}}$ at $q = 0\,\mathrm{e}$ for atomic displacements $dr$ (red) of the oxygen atom and the $-F$ contribution at $dr = 0\,\text{Å}$ for different charges (blue). The lines in the top plot are 2$^{\mathrm{nd}}$-order polynomial fits of the data in the scatter plots. We show the corresponding derivatives in the bottom plot, showing satisfactory agreement at $dq = dr = 0$, as indicated by the crossing point of red and blue lines.

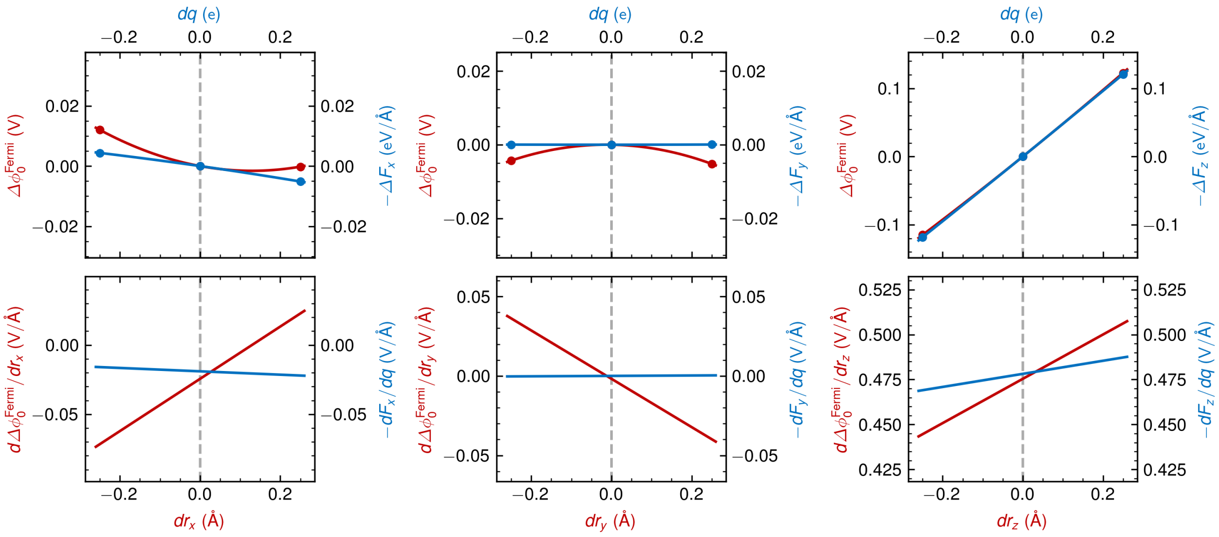


Figure S4: Equivalent figure to S3, except we investigate the twofold bridge adsorption site on the Cu(100) surface.

Using the relation in eq. (S32), we describe the Born effective charges $\mathbf{Z}_i^*$ via

$$\mathbf{Z}_i^* = \varepsilon_0 A \left. \frac{\partial \mathbf{F}_i}{\partial q} \right|_{q=0} . \tag{S33}$$

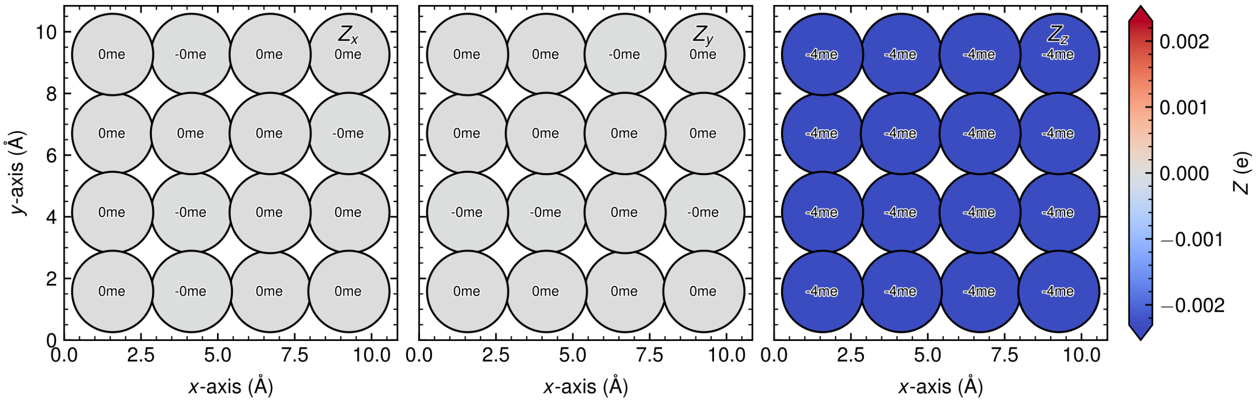


Figure S5: The Born effective charges $\mathbf{Z}_i^* = \varepsilon_0 A \; \partial \mathbf{F}/\partial q$ for the top layer of a clean Cu(100) slab.

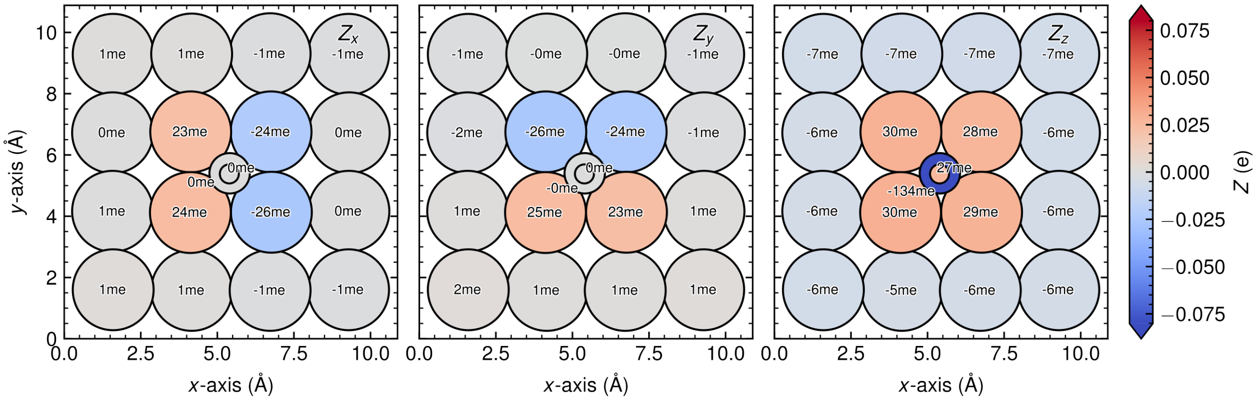


Figure S6: The Born effective charges $\mathbf{Z}_i^* = \varepsilon_0 A\ \partial \mathbf{F}/\partial q$ for the top layer of a Cu(100) slab with one OH adsorbate in the hollow site.

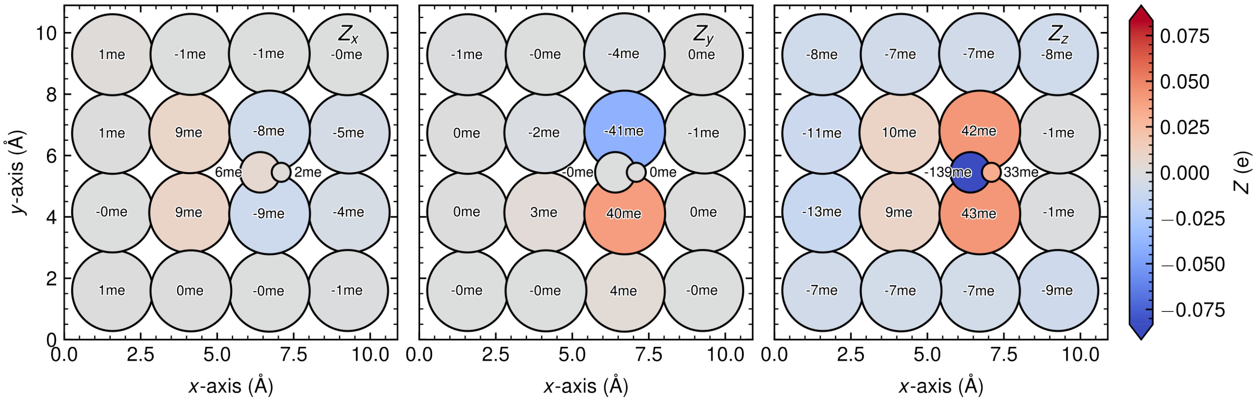


Figure S7: The Born effective charges $\mathbf{Z}_i^* = \varepsilon_0 A\ \partial \mathbf{F}/\partial q$ for the top layer of a Cu(100) slab with one OH adsorbate in the bridge site.

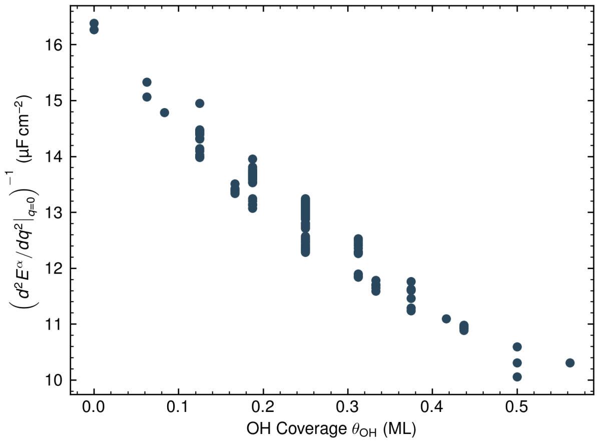


Figure S8: The electronic capacitance contribution $C_{\mathrm{el},0}$, i.e. the inverse second derivative of the structure energy with respect to the excess surface charge $q$, versus the surface coverage $\theta$.

## SIV.3 Machine Learning the Cu(100) System

### SIV.3.1 Energies and Forces at the PZC

To train a suitable Cu – O – H machine-learned interatomic potential (MLIP), we iteratively created a data set using the `wfl` package[19]. We start from a small dataset of isolated atoms, dimers of different bond length, scaled bulk copper oxides and hydrides, and a few Cu(100) slab structures. After training a MACE model on this data set, we generate new structures using MD and optimization simulations. Then, using furthest point sampling, we select roughly 30 structures each generation, calculate these structures in DFT, and then retrain our model. In total, our data set consists of 369 structures and is available at (URL will be filled in after acceptance). We show the training and testing errors in Fig. S9.

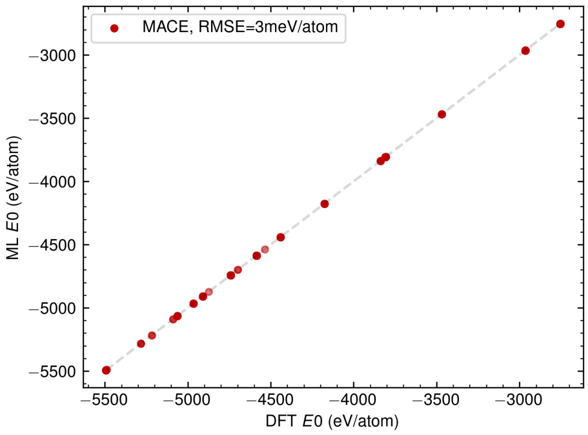


(a) $E_0/n_{\mathrm{atoms}}$ error for the training set.

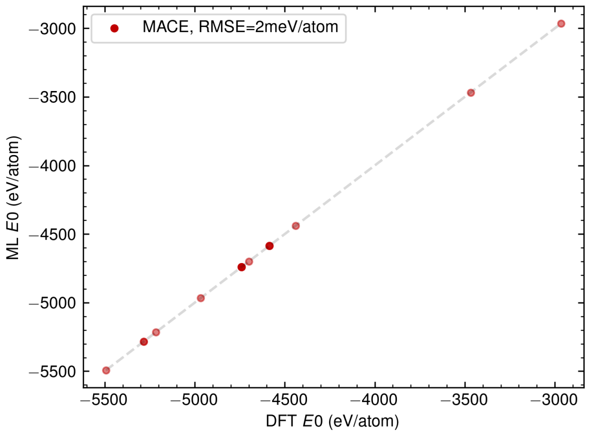


(b) $E_0/n_{\mathrm{atoms}}$ error for the test set.

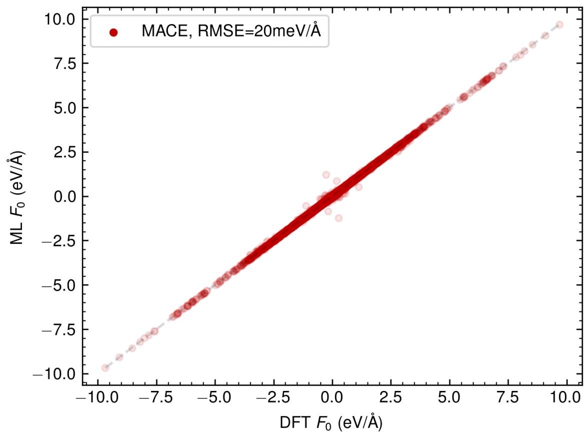


(c) $F_0$ error for the training set.

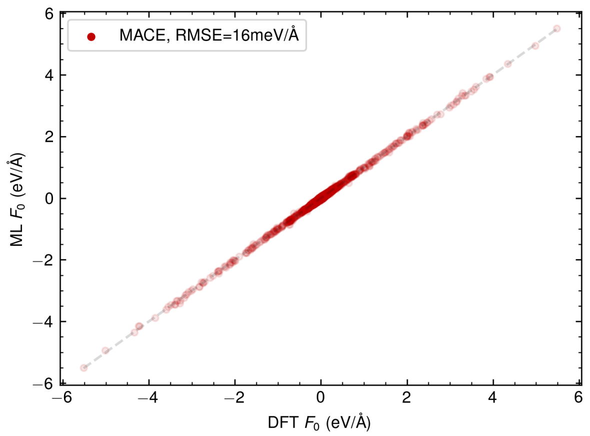


(d) $F_0$ error for the test set.

Figure S9: $E$ and $F$ errors for our MACE ML potential. The total structure set consists of 369 structures. 90% of the data set went into the training set, and 10% went into the test set.

### SIV.3.2 Surface Dipole Moment and Born Effective Charges

The data set for the $P_z$ and $\mathbf{Z}_i^*$ learning consists of 195 symmetrically unique, optimized Cu(100) symmetric slab setups with different coverages of OH adsorbates on the hollow and bridge adsorption sites. As the symmetric slab setup results in an inversion of the $\mathbf{Z}_i^*$ vectors for all atoms below the cell middle, we train only on the atoms belonging to the top half of the cell.

We train our $z$-oriented $P_z$ and $\mathbf{Z}_i^*$ model by augmenting the NequIP[8] code as described in the main text. The descriptor cutoff was set to 4 Å with 1 interaction block (hyperparameter `num_layers=1`). We found the network to be satisfactorily converged after 1000 epochs. The total configuration file

is provided as an external file.

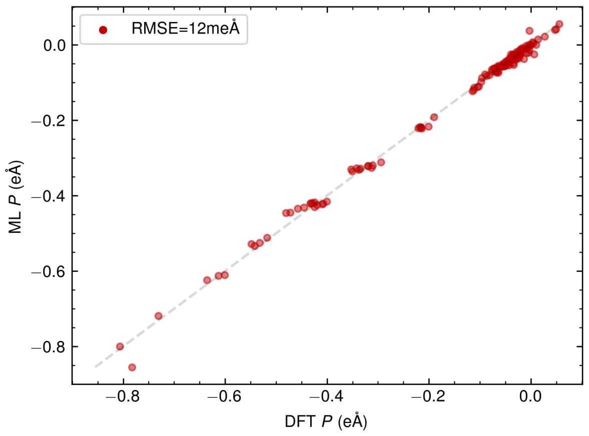


(a) $P_z$ error for the training set.

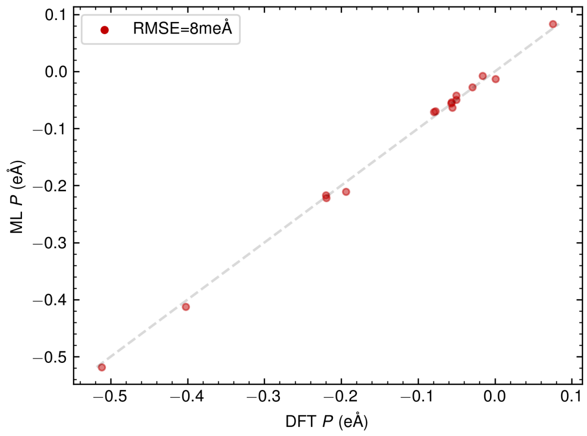


(b) $P_z$ error for the test set.

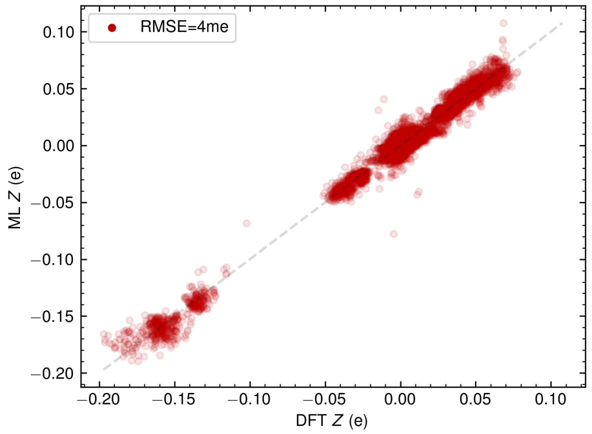


(c) $\mathbf{Z}_i^*$ error for the training set.

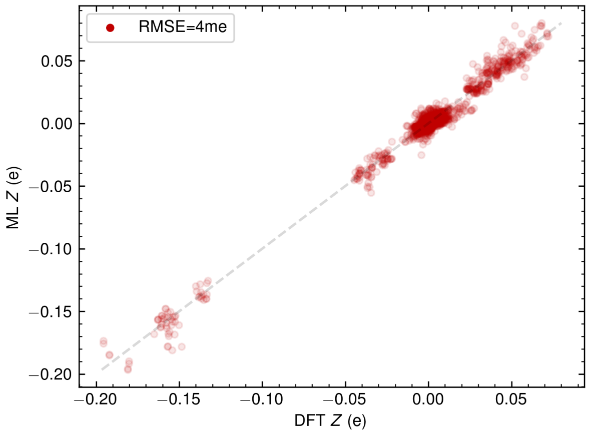


(d) $\mathbf{Z}_i^*$ error for the test set.

Figure S10: Training (90% of the data set) and test (10%) errors for the $P_z$ and $\mathbf{Z}_i^*$ prediction of the Cu(100)-OH system.

To get the work function $\phi_0$ we transformed $P_z$ using eq. (S31). As a reference work function we used the clean Cu(100) surface, which had a value of $\phi_0^{\mathrm{ref}} = 4.24\,\mathrm{V}$.

## SIV.4 Free Energy Contributions

### SIV.4.1 Adsorbate Contributions

Using the ASE HarmonicThermo package[7], we calculate the free energy corrections within the harmonic approximation for OH adsorbed on Cu(100). We find almost identical values for the

bridge and hollow site, as shown in table S1.

Table S1: PBE vibrational energy terms for OH on Cu(100) at $T = 298.15\,\mathrm{K}$ in an implicit solvent environment.

| Ads. Site | $E_{\mathrm{ZPE}}^{*\mathrm{OH}}$ | $H^{*\mathrm{OH}}$ | $TS_{\mathrm{vib}}^{*\mathrm{OH}}$ | $(H^{*\mathrm{OH}} - TS_{\mathrm{vib}}^{*\mathrm{OH}})$ |
|---|---|---|---|---|
| Hollow | 0.344 eV | 0.398 eV | 0.097 eV | 0.301 eV |
| Bridge | 0.353 eV | 0.404 eV | 0.098 eV | 0.306 eV |

By combining the values in Table S1 with the predictions of $\phi_0$ and the calculated capacitance $C_{\mathrm{el},0}$ (Table S2) we can thus calculate free energies $F_0^{\alpha}$. We show a selection of relevant configurations in Table S3.

Table S2: The work function and the area-normalized interfacial capacitance for the adsorbed OH on Cu(100) in an implicit solvent environment. We show both the DFT-calculated values as well as the machine-learned predicted values of $\phi_0$.

| Configuration $\alpha$ | $\phi_0^{\mathrm{DFT}}$ (V) | $\phi_0^{\mathrm{ML}}$ (V) | $C_{\mathrm{el},0}^{\mathrm{DFT}}/(2A)$ (μF cm$^{-2}$) |
|---|---|---|---|
| Clean | 4.240 | 4.240 | 16.270 |
| $p(4\times4)$ Hollow | 4.061 | 4.047 | 15.079 |
| $p(4\times4)$ Bridge | 4.197 | 4.200 | 15.384 |
| $c(2\times2)$ Hollow | 2.848 | 2.863 | 10.638 |
| $c(2\times2)$ Bridge | 4.370 | 4.375 | 10.300 |

Table S3: The potential and free energy for adsorbed OH on Cu(100) at $T = 298.15\,\mathrm{K}$ in an implicit solvent environment and a symmetric cell setup. We show the DFT-calculated values as well as the machine-learned prediction.

| Configuration $\alpha$ | $n_{\mathrm{Cu}}$ | $n_{\mathrm{OH}}$ | $n_{\mathrm{sites}}$ | $E_0^{\mathrm{DFT}}$ (eV) | $E_0^{\mathrm{ML}}$ (eV) | $F_0^{\mathrm{DFT}}$ (eV/Å) | $F_0^{\mathrm{ML}}$ (eV/Å) |
|---|---|---|---|---|---|---|---|
| Clean | 96 | 0 | 32 | -527380.030 | -527380.125 | -527380.030 | -527380.125 |
| $p(4\times4)$ Hollow | 96 | 2 | 32 | -528291.928 | -528291.938 | -528291.326 | -528291.336 |
| $p(4\times4)$ Bridge | 96 | 2 | 32 | -528291.799 | -528291.812 | -528291.187 | -528291.201 |
| $c(2\times2)$ Hollow | 96 | 16 | 32 | -534672.350 | -534672.312 | -534667.534 | -534667.496 |
| $c(2\times2)$ Bridge | 96 | 16 | 32 | -534673.782 | -534673.875 | -534668.886 | -534668.979 |

### SIV.4.2 OH Chemical Potential Contributions

We calculate $G^{\mathrm{ref}}_{\mathrm{H_2O}}$ and $G^{\mathrm{ref}}_{\mathrm{H_2}}$ by optimizing the geometry of the molecules and calculating free energy corrections with the ASE IdealGasThermo package (Table S4).

Table S4: DFT relaxation results for the molecule relaxations using the PBE exchange-correlation functional. $E^{\mathrm{molecule}}$ is the relaxed DFT energy of the molecule. Additionally, we show the vibrational energy terms for the gas-phase molecules at $T = 298.15\,\mathrm{K}$ and $p = 1 \times 10^5\,\mathrm{Pa}$ (For $H_2O$: $p = 3500\,\mathrm{Pa}$).

| Molecule | $E^{\mathrm{molecule}}$ (eV) | $E_{\mathrm{ZPE}}$ (eV) | $H$ (eV) | $TS$ (eV) | $G^{\mathrm{ref}}$ (eV) |
|---|---|---|---|---|---|
| $H_2O$ | −471.667 | 0.577 | 0.677 | 0.671 | −471.084 |
| $H_2$ | −31.705 | 0.391 | 0.474 | 0.404 | −31.244 |

We thus obtain $\mu^{\circ}_{\mathrm{OH}} = -455.843\,\mathrm{eV}$ at $T = 300\,\mathrm{K}$.

## SIV.5 Molecular Dynamics of adsorbed OH on Cu(100)

### SIV.5.1 Double-Well Correction via Maxwell Construction

Normally, the equilibrium condition in eq. (S17) only has one solution, thus providing the singular value $Q$ in eq. (S19) used to obtain $\Omega^{Z_i}(\phi_{\mathrm{E}})$. However, in some cases we find $\phi_{\mathrm{E}}$ ranges where the formation energy $\tilde{F}^{Z_i}(q, \phi_{\mathrm{E}})$ becomes a double-well potential, exhibiting two minima in the variable $q$ (see Fig. S11). In this case, "blindly" following eqs. (S13) and (S16) for all sampled values $Q$ leads to a seemingly multivalued function $\Omega^{Z_i}(Q_i(\phi_{\mathrm{E}}))$, as multiple charge values $Q_i$ fulfill eq. (S17) (see Fig. S12) and are thus mapped onto a single potential value $\phi_{\mathrm{E}}$.

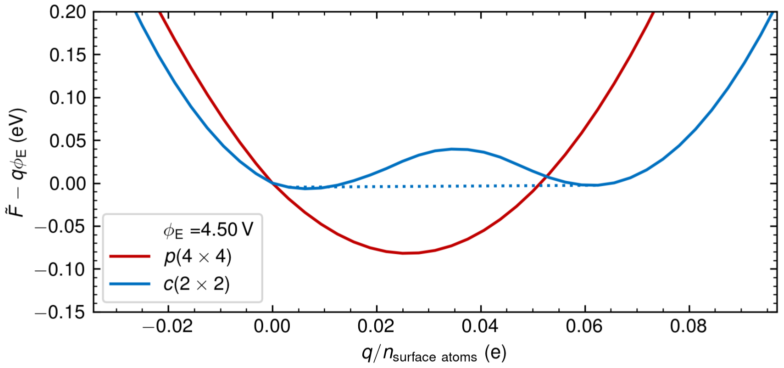


Figure S11: Plot of $\tilde{F}(q,\phi_{\text{E}})$ (eq. (S16)) at different test conditions. In most cases, e.g. the $p(4\times4)$ ensemble, $\tilde{F}(q,\phi_{\text{E}})$ yields only one minimum value and thus only one solution of eq. (S17). In this case a one-to-one mapping of $Q$ to $\phi_{\text{E}}$ exists. However, for ensembles where $\tilde{F}(q,\phi_{\text{E}})$ (eq. (S16)) is a double-well potential, it exhibits two (local) minima (e.g. the $c(2\times2)$ ensemble). As a result, if the minimum condition is evaluated via setting the derivative in $q$ to zero (cf. eq. (S17)) two solutions will emerge. Both fulfill the (weaker) equilibrium criterion that system-internal and externally applied potential are equal ($\langle\phi\rangle|_Q = \phi_{\text{E}}$, cf. eq. (S17)). The true equilibrium solution can be deduced by choosing only the global minimum or performing a Maxwell construction on $F(q)$ (dashed lines, see text). The systems shown here is a $NVT$ molecular dynamics simulated Cu(100) electrode with different OH coverages at different values $q$ using the above described RAZOR MLIP.

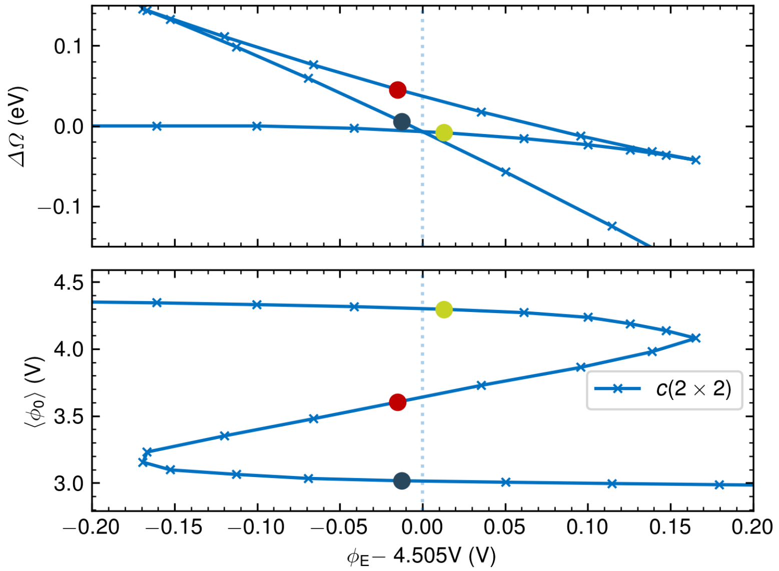


Figure S12: We show the consequence of the double-well situation shown in Fig. S11: Multiple values $Q_i$ (shown as the "x" markers) correspond to the same value $\phi_{\text{E}}$ when using eq. (S17). Simultaneously, we show the validity of using a Maxwell construction, as the minimum $\Omega$ path goes through the bisection of the "S" shape in the curve below.

While several, somewhat equivalent strategies can be applied to circumvent this problem, here we solve this issue by applying a Maxwell construction to $F(q)$.

### SIV.5.2 Other Molecular Dynamics Results

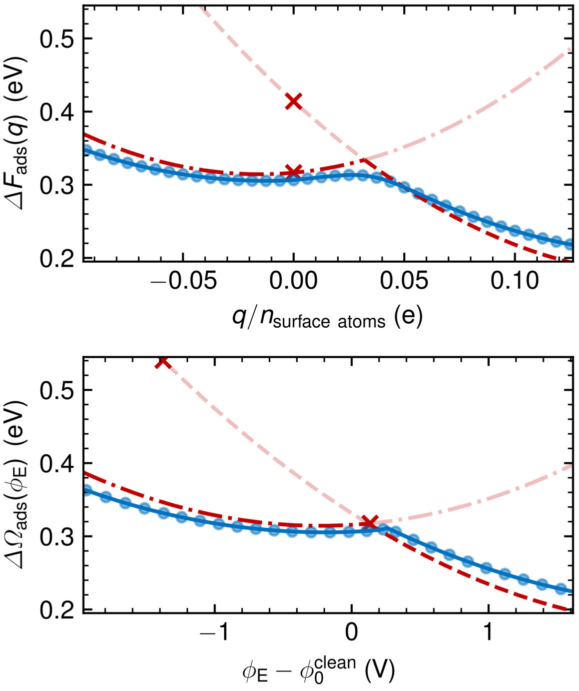


Figure S13: Adsorption free energy change $\Delta F^{\circ}_{\mathrm{ads}}(q)$ (upper panel) and constant-potential grand-canonical adsorption free energy change $\Delta\Omega^{\circ}_{\mathrm{ads}}(\phi_{\mathrm{E}})$ (lower panel) for 0.5 ML OH-covered Cu(100) surfaces. Compared are RAZOR-MLIP based molecular dynamics simulations (blue circles, line added to guide the eye) to DL-corrected *ab initio* thermodynamics of $T = 0\,\mathrm{K}$ $c(2\times2)$-$\mathrm{OH_{Hollow}}$ (red dashed line) and $c(2\times2)$-$\mathrm{OH_{Bridge}}$ (red dashed dotted line) adsorbate structures. The red crosses mark the $q$ values at which we perform the free energy evaluations.

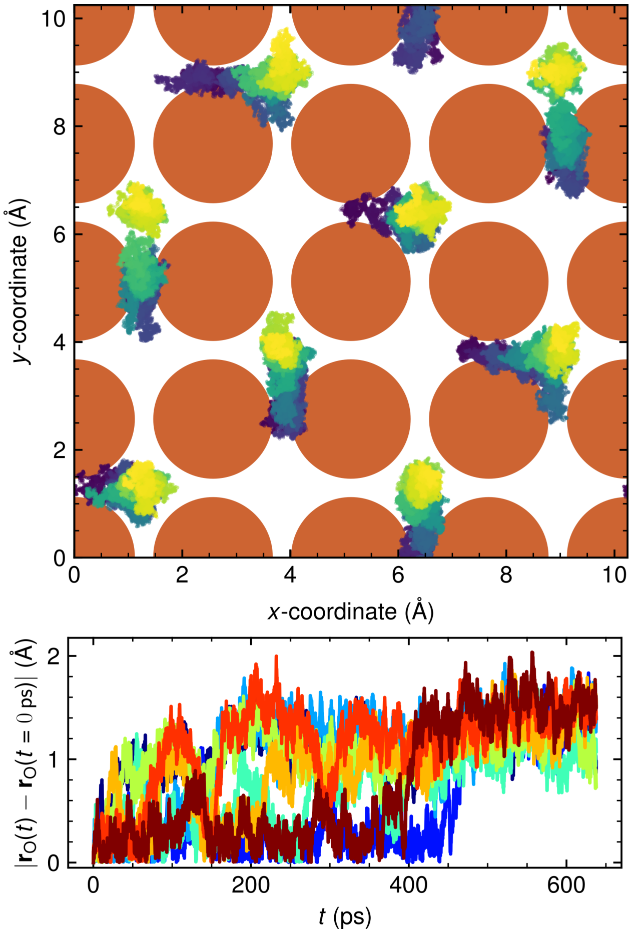


Figure S14: Structural results from a RAZOR-MD run at a surface bias charge $q = 0.0625\,\mathrm{e}$ per surface Cu atom. The MD is initialized with the $c(2 \times 2)$-OH adsorbed in the twofold bridge sites (dark blue scatter points, upper plot) and the bias drives the adsorbates into the fourfold hollow sites (yellow scatter points at later times, upper plot). However, this process is quite slow, as can be seen in the bottom panel. Here, we show the distance of the different adsorbate positions $\mathbf{r_i}$ at every time $t$ versus the starting position $\mathbf{r_i}(t = 0\,\mathrm{ps})$. We observe that the diffusion step of the last adsorbate into the hollow site occurs at $450\,\mathrm{ps}$, thus finally creating the more stable $(c2 \times 2)$-hollow configuration.

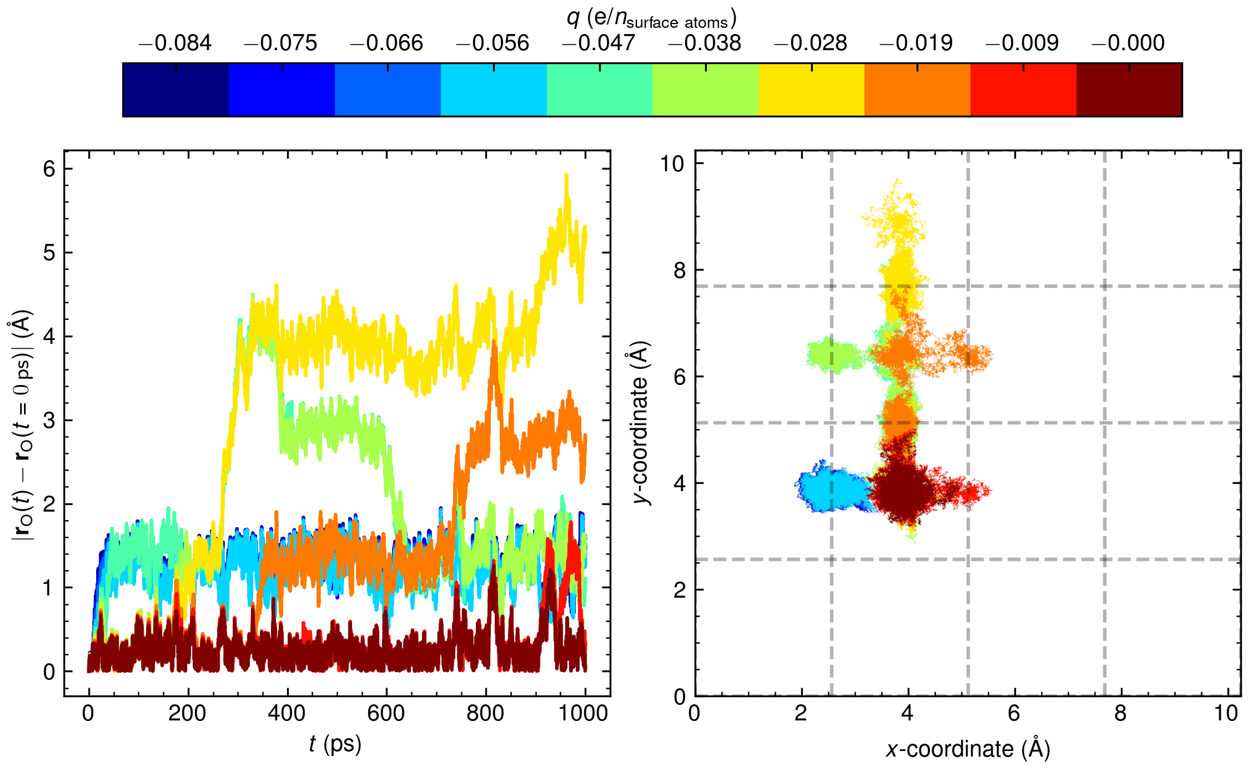


Figure S15: The mobility of an adsorbed OH molecule on a $(4 \times 4)$ Cu(100) cell as calculated via RAZOR-MLIP MD simulations at $T = 300\,\mathrm{K}$. On the left, we show the distance of the oxygen atom relative to the initial position in the fourfold hollow site as a function of the simulation time $t$. On the right, we plot the $x - y$ position of the O atom throughout the MD simulation. We observe that at positive $q$, the OH remains at the initial hollow site and does not diffuse away. At very negative $q$ it only diffuses once to a neighboring bridge site and remains there. In the intermediate region, multiple diffusion steps are possible and occur. We show that a sampling of at least multiple hundred ps is necessary to observe any diffusion steps, highlighting the need for computationally efficient evaluations such as RAZOR-MLIP.

# SV Modeling $H_2O$ in an Electric Field

## SV.1 Machine Learning $H_2O$

The data set for learning $H_2O$'s energetic properties consists of 1018 $H_2O$ molecules which we randomly rotated. Furthermore, we randomly distort the H – O bond lengths and the H – O – H angle.

### SV.1.1 Energies and Forces for the field free case

We trained $E_0$ and $F_0$ using the NequIP architecture[8]. We set the cutoff radius to 4 Å, with one interaction block, and $l_{\max} = 1$. We found the network to be satisfactorily converged after 1000 epochs.

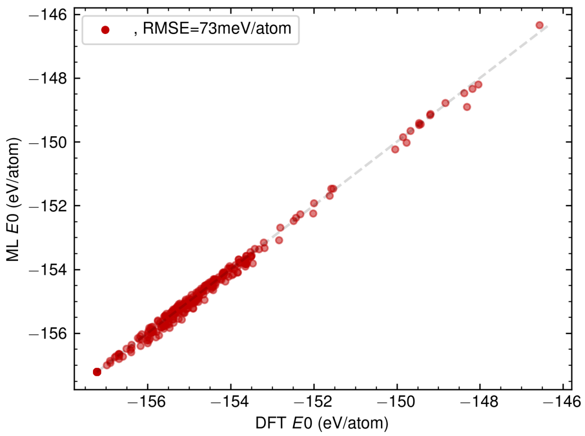


(a) $E_0/n_{\text{atoms}}$ error for the training set.

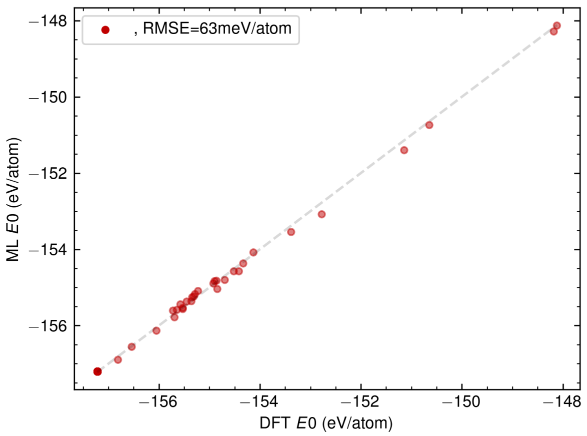


(b) $E_0/n_{\text{atoms}}$ error for the test set.

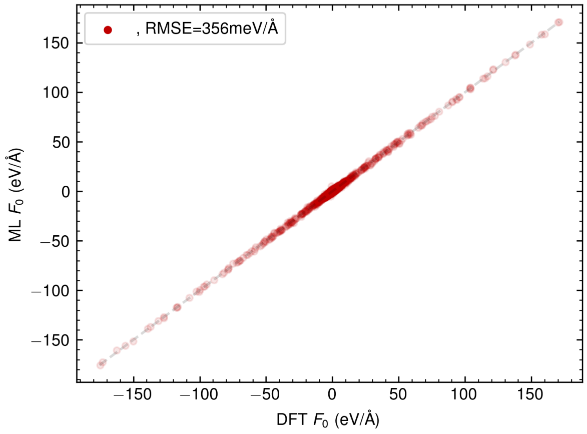


(c) $F_0$ error for the training set.

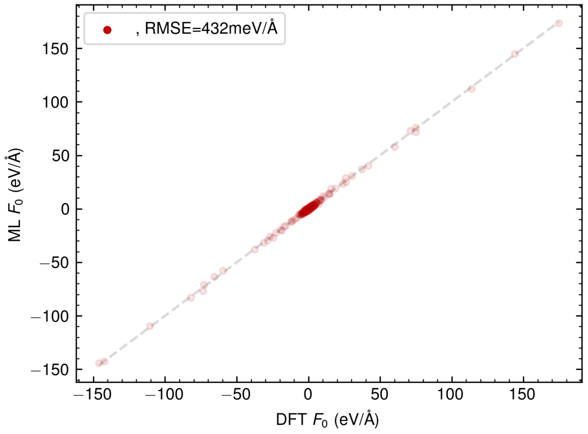


(d) $F_0$ error for the test set.

Figure S16: $E$ and $F$ errors for our $H_2O$ NequIP ML potential. The total structure set consists of 1018 structures. 90% of the data set went into the training set, and 10% went into the test set.

### SV.1.2 Surface Dipole Moment and Born Effective Charges

To determine $P_z$ and $\mathbf{Z}_i^*$ we run DFT evaluations at different applied electric fields within the ESM scheme in Quantum ESPRESSO[5], noting that the input parameter `esm_efield` is only the true

applied $E_z$ for $P_z = 0$. Instead the applied $E_z$ is recomputed *a posteriori* from the spatial derivative of the electrostatic potential along the $z$-coordinate far from the atomic region (the slopes in Fig. S17). Furthermore, for a true $E_z = 0$ reference, we evaluate the molecule not within metal-slab-metal boundary conditions ("bc2"), but in open boundary conditions ("bc1"), thus guaranteeing that the potential slope is 0.

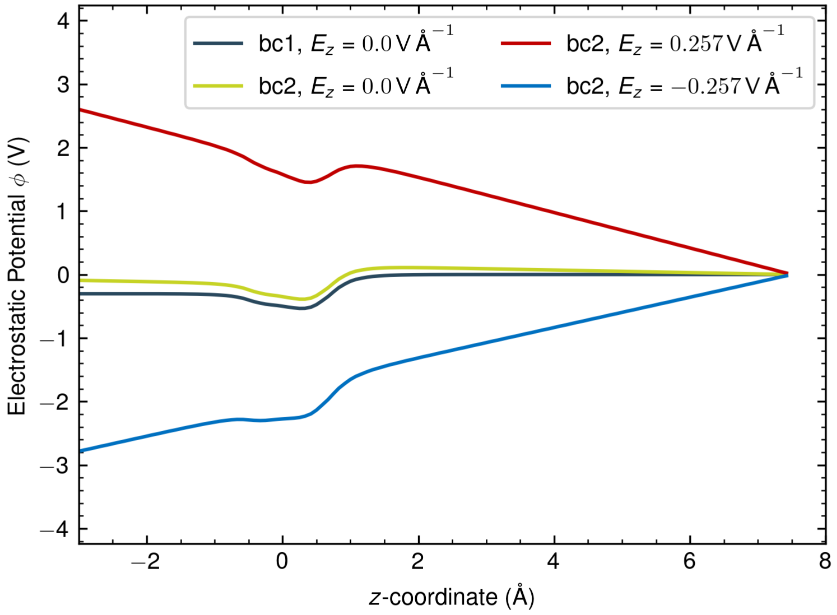


Figure S17: DFT $xy$-averaged electrostatic potential versus the $z$-coordinate in different ESM setups. We see that although we do not include an $E$ field, the "bc2" calculations nevertheless include a potential drop. We remedy this by using the open boundary condition calculations "bc1" as a reference.

Thus, we train our MLIP on the derivatives $\partial E/\partial E_z$ and $\partial F/\partial E_z$ at $E_z = 0$ by running three DFT evaluations ($E_z \in \{-0.257\,\mathrm{V\,Å^{-1}}, 0\,\mathrm{V\,Å^{-1}}, 0.257\,\mathrm{V\,Å^{-1}}\}$) and then taking the derivative of a fitted quadratic polynomial.

We train our $z$-oriented $P$ and $Z$ model by augmenting the NeQUIP[8] code as described in the main text. The descriptor cutoff was set to 4 Å with 1 interaction block (hyperparameter `num_layers=1`) and $l_{\max} = 1$. We found the network to be satisfactorily converged after 1000 epochs. The total configuration file is provided as an external file.

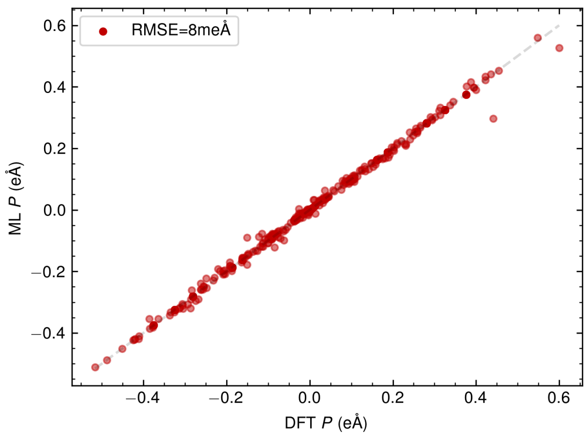


(a) $P_z$ error for the training set.

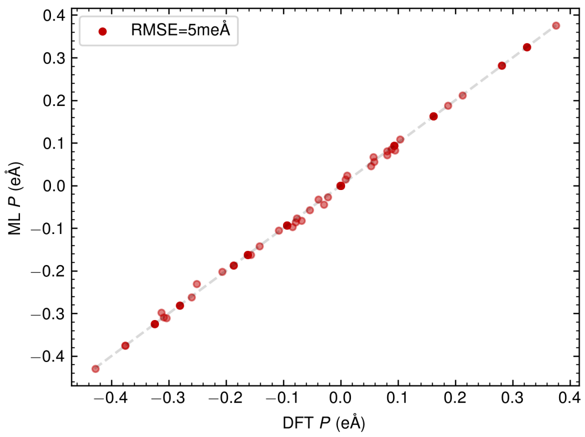


(b) $P_z$ error for the test set.

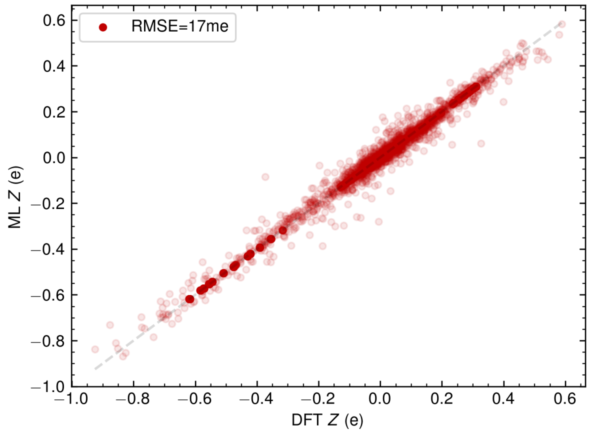


(c) $\mathbf{Z}_i^*$ error for the training set.

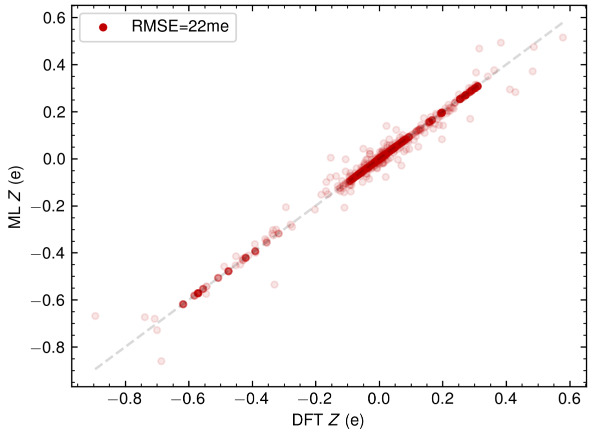


(d) $\mathbf{Z}_i^*$ error for the test set.

Figure S18: Training (90% of the data set) and test (10%) errors for the $P_z$ and $\mathbf{Z}_i$ prediction for the single $H_2O$ molecule.

## SV.2 $H_2O$: Importance of $z$-projection in learning $P_z$

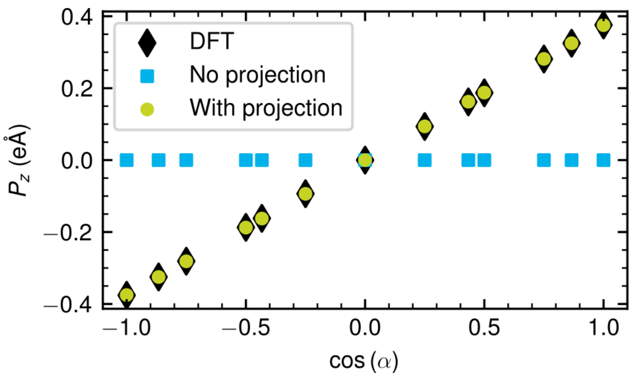


Figure S19: We show the relevance of including the $z$-projection in the ML approach as described in the main text. With the projection, and the thus introduced rotational equivariance of $P_z$ to $E_z$, we recreate the DFT $P_z$ values. Without the projection, the atomic representation is rotationally invariant, thus we consistently predict the identical value, no matter the orientation of $P_z$ to $E_z$.

## SV.3 Geometry Optimization of $H_2O$ at an Applied Electric Field

Using eq. (S3), we run geometry relaxations for a range of $E_z$ values. In Fig. S20, we show the field-dependent behavior of different observables.

Increasing the electric field to $3\,\mathrm{V\,Å}^{-1}$ decreases the H–O–H angle by $5\,\%$ and increases H–O distance by $1\,\%$. This "sharpening" of the molecule leads to an increased dipole moment of $5\,\%$. Comparing our model to a point charge model, choosing point charges that match the dipole moment at $E_z = 0\,\mathrm{V\,Å}^{-1}$, we report that there is virtually no difference in the dipole-field interaction energy at $E_z = 3\,\mathrm{V\,Å}^{-1}$ ($\Delta = 5\,\mathrm{meV} \approx 4\,\%$).

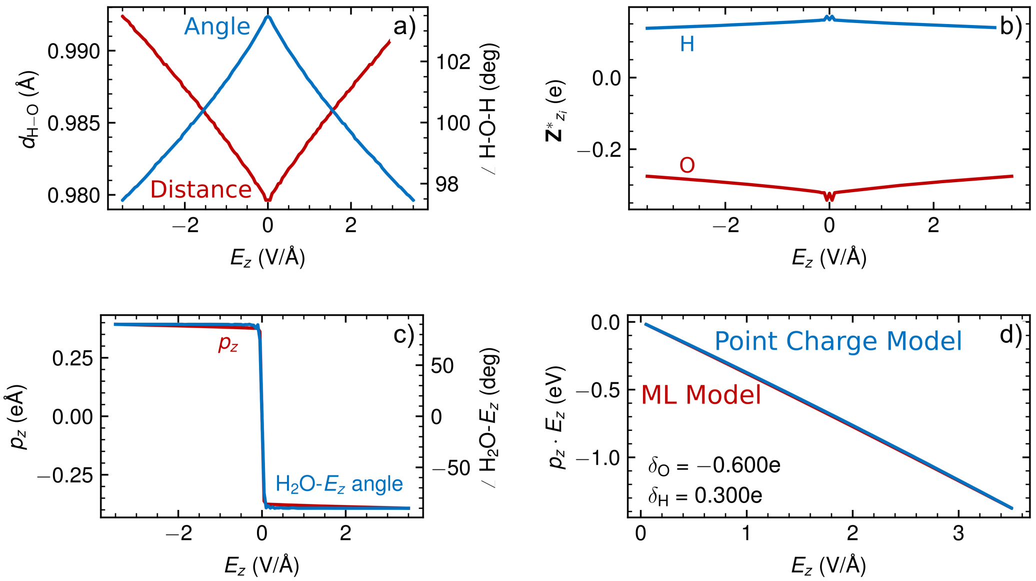


Figure S20: $H_2O$ geometry relaxation results at different applied electric fields $E_z$: a) the H−O bond distance in red and the H−O−H angle in blue; b) the Born effective charges on the hydrogen (blue) and oxygen (red) atoms; c) $H_2O$'s dipole moment $P_z$ (red) and the angle between $H_2O$'s $C_2$ rotational axis and the $E_z$ vector (blue); d) the dipole-field interaction as predicted by our ML model (red) versus a point charge model (blue).

## SV.4 Molecular Dynamics of a $H_2O$ Molecule in an Electric Field

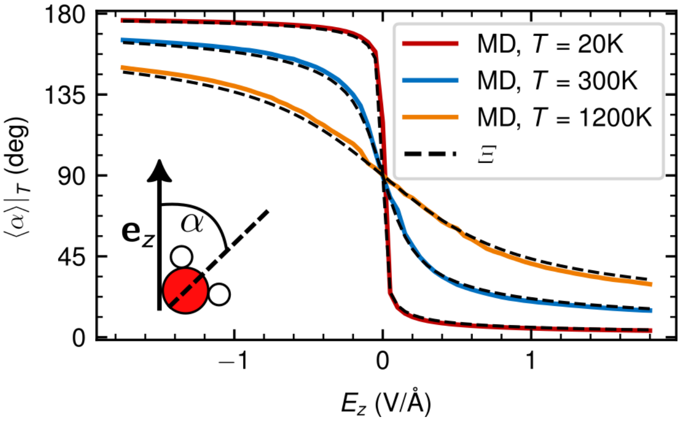


Figure S21: Average angle $\langle\alpha\rangle$ between the molecular dipole axis of an isolated $H_2O$ molecule and an applied electric field as a function of the electric field strength $E_z$. Compared are results from $NVT$ molecular dynamics simulations based on the augmented MLIP at different temperatures with the analytic partition function $\Xi$ from Ref.[20].

To demonstrate RAZOR, we investigate a single rotating $H_2O$ molecule in the presence of a homogeneous electric field $E_z$. Predicting $P_z$ for different molecular geometries and orientations and combining it with the baseline energetics $E_0$ allows the computation of thermal averages via MD runs at given temperature $T$ and field strength $E_z$ (see Fig. S21). The agreement between according simulations with the analytical, theoretical result based on the (classical) partition function of a freely rotating dipole[20] proves the accuracy of RAZOR and shows that vibration-induced changes of the $H_2O$ dipole moment are only minute up to very high temperatures.

## SV.5 $H_2O$ slab

We report further analyses on learning the polarization of extended water slabs in vacuum (cf. Fig. S22). We find that RAZOR predicts the total dipole moment with mean absolute relative errors of 9% relative to the DFT reference, while an (optimized) point charge model, as in non-polarizable, classical force fields yields offsets of 62%. The superior behavior of RAZOR is linked to its intrinsic ability to describe local-environment dependent, Born effective charges which is very important in highly polarizable, condensed water[21–23].

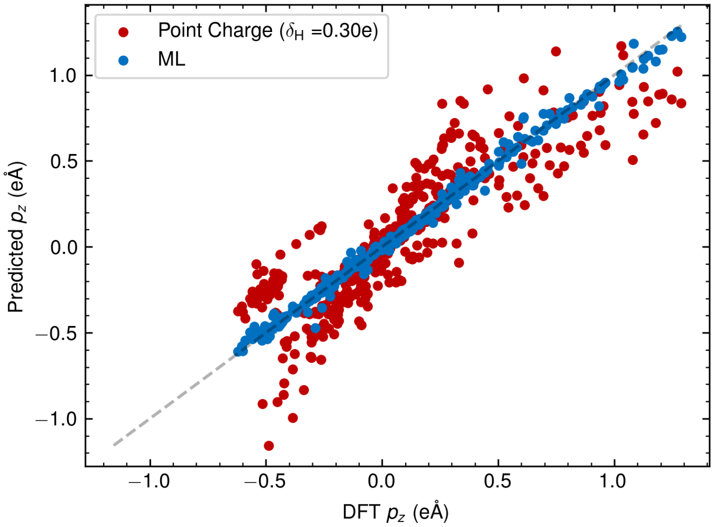


Figure S22: The DFT-calculated polarization of different $H_2O$ slabs (32 $H_2O$ molecules per structure) versus our ML-model (blue) versus a standard point charge model with $\delta_H = 0.3\,e$ and $\delta_O = -0.6\,e$ (cf. Fig. S20). Mean absolute errors: ML model = 7 meÅ, Point charge model = 59 meÅ.

# References


(1) Giannozzi, P.; Baroni, S.; Bonini, N.; Calandra, M.; Car, R.; Cavazzoni, C.; Ceresoli, D.; Chiarotti, G. L.; Cococcioni, M.; Dabo, I.; Corso, A. D.; de Gironcoli, S.; Fabris, S.; Fratesi, G.; Gebauer, R.; Gerstmann, U.; Gougoussis, C.; Kokalj, A.; Lazzeri, M.; Martin-Samos, L.; Marzari, N.; Mauri, F.; Mazzarello, R.; Paolini, S.; Pasquarello, A.; Paulatto, L.; Sbraccia, C.; Scandolo, S.; Sclauzero, G.; Seitsonen, A. P.; Smogunov, A.; Umari, P.; Wentzcovitch, R. M. QUANTUM ESPRESSO: a modular and open-source software project for quantum simulations of materials. *Journal of Physics: Condensed Matter* **2009**, *21*, 395502, DOI: 10.1088/0953-8984/21/39/395502.

(2) Giannozzi, P.; Andreussi, O.; Brumme, T.; Bunau, O.; Nardelli, M. B.; Calandra, M.; Car, R.; Cavazzoni, C.; Ceresoli, D.; Cococcioni, M.; Colonna, N.; Carnimeo, I.; Corso, A. D.; de Gironcoli, S.; Delugas, P.; DiStasio, R. A.; Ferretti, A.; Floris, A.; Fratesi, G.; Fugallo, G.; Gebauer, R.; Gerstmann, U.; Giustino, F.; Gorni, T.; Jia, J.; Kawamura, M.; Ko, H.-Y.; Kokalj, A.; Küçükbenli, E.; Lazzeri, M.; Marsili, M.; Marzari, N.; Mauri, F.; Nguyen, N. L.; Nguyen, H.-V.; de-la Roza, A. O.; Paulatto, L.; Poncé, S.; Rocca, D.; Sabatini, R.; Santra, B.; Schlipf, M.; Seitsonen, A. P.; Smogunov, A.; Timrov, I.; Thonhauser, T.; Umari, P.; Vast, N.; Wu, X.; Baroni, S. Advanced capabilities for materials modelling with Quantum ESPRESSO. *Journal of Physics: Condensed Matter* **2017**, *29*, 465901, DOI: 10.1088/1361-648X/aa8f79.

(3) Perdew, J. P.; Burke, K.; Ernzerhof, M. Generalized Gradient Approximation Made Simple. *Physical Review Letters* **1996**, *77*, 3865–3868, DOI: 10.1103/PhysRevLett.77.3865.

(4) Garrity, K. F.; Bennett, J. W.; Rabe, K. M.; Vanderbilt, D. Pseudopotentials for high-throughput DFT calculations. *Computational Materials Science* **2014**, *81*, 446–452, DOI: https://doi.org/10.1016/j.commatsci.2013.08.053.

(5) Otani, M.; Sugino, O. First-principles calculations of charged surfaces and interfaces: A plane-

wave nonrepeated slab approach. *Physical Review B* **2006**, *73*, 115407, DOI: 10.1103/PhysRevB.73.115407.

(6) Andreussi, O.; Dabo, I.; Marzari, N. Revised self-consistent continuum solvation in electronic-structure calculations. *The Journal of Chemical Physics* **2012**, *136*, 064102, DOI: 10.1063/1.3676407.

(7) Hjorth Larsen, A.; Jørgen Mortensen, J.; Blomqvist, J.; Castelli, I. E.; Christensen, R.; Dułak, M.; Friis, J.; Groves, M. N.; Hammer, B.; Hargus, C.; Hermes, E. D.; Jennings, P. C.; Bjerre Jensen, P.; Kermode, J.; Kitchin, J. R.; Leonhard Kolsbjerg, E.; Kubal, J.; Kaasbjerg, K.; Lysgaard, S.; Bergmann Maronsson, J.; Maxson, T.; Olsen, T.; Pastewka, L.; Peterson, A.; Rostgaard, C.; Schiøtz, J.; Schütt, O.; Strange, M.; Thygesen, K. S.; Vegge, T.; Vilhelmsen, L.; Walter, M.; Zeng, Z.; Jacobsen, K. W. The atomic simulation environment—a Python library for working with atoms. *Journal of Physics: Condensed Matter* **2017**, *29*, 273002, DOI: 10.1088/1361-648X/aa680e.

(8) Batzner, S.; Musaelian, A.; Sun, L.; Geiger, M.; Mailoa, J. P.; Kornbluth, M.; Molinari, N.; Smidt, T. E.; Kozinsky, B. E(3)-equivariant graph neural networks for data-efficient and accurate interatomic potentials. *Nat Commun* **2022**, *13*, 2453, DOI: 10.1038/s41467-022-29939-5.

(9) Gigli, L.; Veit, M.; Kotiuga, M.; Pizzi, G.; Marzari, N.; Ceriotti, M. Thermodynamics and dielectric response of BaTiO3 by data-driven modeling. *npj Comput Mater* **2022**, *8*, 209, DOI: 10.1038/s41524-022-00845-0.

(10) Dudzinski, A. M.; Diesen, E.; Heenen, H. H.; Bukas, V. J.; Reuter, K. First Step of the Oxygen Reduction Reaction on Au(111): A Computational Study of O2 Adsorption at the Electrified Metal/Water Interface. *ACS Catalysis* **2023**, *13*, 12074–12081, DOI: 10.1021/acscatal.3c02129.

(11) Hörmann, N. G.; Marzari, N.; Reuter, K. Electrosorption at metal surfaces from first principles. *npj Computational Materials* **2020**, *6*, 136, DOI: 10.1038/s41524-020-00394-4.

(12) Rogal, J.; Reuter, K. Ab initio atomistic thermodynamics for surfaces: A primer. *Experiment, Modeling and Simulation of Gas-Surface Interactions for Reactive flows in Hypersonic Flights* **2007**, *14*, 2–1.

(13) Bergmann, N.; Hörmann, N. G.; Reuter, K. Ab Initio-Based Modeling of Thermodynamic Cyclic Voltammograms: A Benchmark Study on Ag(100) in Bromide Solutions. *Journal of Chemical Theory and Computation* **2023**, *19*, 8815–8825, DOI: 10.1021/acs.jctc.3c00957, PMID: 38038493.

(14) Nørskov, J. K.; Rossmeisl, J.; Logadottir, A.; Lindqvist, L.; Kitchin, J. R.; Bligaard, T.; Jónsson, H. Origin of the Overpotential for Oxygen Reduction at a Fuel-Cell Cathode. *The Journal of Physical Chemistry B* **2004**, *108*, 17886–17892, DOI: 10.1021/jp047349j.

(15) Hörmann, N. G.; Andreussi, O.; Marzari, N. Grand canonical simulations of electrochemical interfaces in implicit solvation models. *The Journal of Chemical Physics* **2019**, *150*, 041730, DOI: 10.1063/1.5054580.

(16) Beinlich, S. D.; Kastlunger, G.; Reuter, K.; Hörmann, N. G. A theoretical investigation of the grand-and the canonical potential energy surface: the interplay between electronic and geometric response at electrified interfaces. *arXiv preprint arXiv:2307.09817* **2023**,

(17) Li, W.-X.; Stampfl, C.; Scheffler, M. Oxygen adsorption on Ag (111): A density-functional theory investigation. *Physical Review B* **2002**, *65*, 075407.

(18) Beinlich, S. D.; Hörmann, N. G.; Reuter, K. Field effects at protruding defect sites in electrocatalysis at metal electrodes? *ACS Catalysis* **2022**, *12*, 6143–6148.

(19) Gelžinytė, E.; Wengert, S.; Stenczel, T. K.; Heenen, H. H.; Reuter, K.; Csányi, G.; Bernstein, N. wfl Python toolkit for creating machine learning interatomic potentials and related

atomistic simulation workflows. *The Journal of Chemical Physics* **2023**, *159*, 124801, DOI: 10.1063/5.0156845.

(20) Huang, J. Zooming into the Inner Helmholtz Plane of Pt(111)–Aqueous Solution Interfaces: Chemisorbed Water and Partially Charged Ions. *JACS Au* **2023**, *3*, 550–564, DOI: 10.1021/jacsau.2c00650.

(21) Khatib, R.; Kumar, A.; Sanvito, S.; Sulpizi, M.; Cucinotta, C. S. The nanoscale structure of the Pt-water double layer under bias revealed. *Electrochimica Acta* **2021**, *391*, 138875, DOI: https://doi.org/10.1016/j.electacta.2021.138875.

(22) Li, L.; Reuter, K.; Hörmann, N. G. Deciphering the Capacitance of the Pt(111)/Water Interface: A Micro- to Mesoscopic Investigation by AIMD and Implicit Solvation. *ACS Electrochemistry* **2025**, *1*, 186–194, DOI: 10.1021/acselectrochem.4c00062.

(23) Zhu, J.-X.; Cheng, J.; Doblhoff-Dier, K. Dielectric profile at the Pt(111)/water interface. *The Journal of Chemical Physics* **2025**, *162*, 024702, DOI: 10.1063/5.0239284.
